# Supplementary material for: NNNLO gravitational quadratic-in-spin interactions at the quartic order in G
Source: arXiv:2003.07890 source file (2021-07-19)
Supplement: Supplementary file 1 [file appendix.pdf]

## A Graph values

$$\text{Fig. 2(a1.1)} = 12\left(\frac{G^4}{r^6}\vec{S}_1\cdot\vec{n}\,\vec{S}_2\cdot\vec{n}\,m_1^3m_2^2\right) - 4\left(\frac{G^4}{r^6}\vec{S}_1\cdot\vec{S}_2\,m_1^3m_2^2\right), \tag{A.1}$$

$$\text{Fig. 2(a1.2)} = 48\left(\frac{G^4}{r^6}\vec{S}_1\cdot\vec{n}\,\vec{S}_2\cdot\vec{n}\,m_1^3m_2^2\right) - 16\left(\frac{G^4}{r^6}\vec{S}_1\cdot\vec{S}_2\,m_1^3m_2^2\right), \tag{A.2}$$

$$\text{Fig. 2(a2.1)} = 48\left(\frac{G^4}{r^6}\vec{S}_1\cdot\vec{n}\,\vec{S}_2\cdot\vec{n}\,m_1^3m_2^2\right) - 16\left(\frac{G^4}{r^6}\vec{S}_1\cdot\vec{S}_2\,m_1^3m_2^2\right), \tag{A.3}$$

$$\text{Fig. 2(a2.2)} = 96\left(\frac{G^4}{r^6}\vec{S}_1\cdot\vec{n}\,\vec{S}_2\cdot\vec{n}\,m_1^3m_2^2\right) - 32\left(\frac{G^4}{r^6}\vec{S}_1\cdot\vec{S}_2\,m_1^3m_2^2\right), \tag{A.4}$$

$$\text{Fig. 2(a2.3)} = 6\left(\frac{G^4}{r^6}\vec{S}_1\cdot\vec{n}\,\vec{S}_2\cdot\vec{n}\,m_1^3m_2^2\right) - 2\left(\frac{G^4}{r^6}\vec{S}_1\cdot\vec{S}_2\,m_1^3m_2^2\right), \tag{A.5}$$

$$\text{Fig. 2(a3.1)} = 32\left(\frac{G^4}{r^6}\vec{S}_1\cdot\vec{n}\,\vec{S}_2\cdot\vec{n}\,m_1^4m_2\right) - \frac{32}{3}\left(\frac{G^4}{r^6}\vec{S}_1\cdot\vec{S}_2\,m_1^4m_2\right), \tag{A.6}$$

$$\text{Fig. 2(b1.1)} = 8\left(\frac{G^4}{r^6}\vec{S}_1\cdot\vec{S}_2\,m_1^3m_2^2\right) - 16\left(\frac{G^4}{r^6}\vec{S}_1\cdot\vec{n}\,\vec{S}_2\cdot\vec{n}\,m_1^3m_2^2\right), \tag{A.7}$$

$$\text{Fig. 2(b1.2)} = 32\left(\frac{G^4}{r^6}\vec{S}_1\cdot\vec{S}_2\,m_1^3m_2^2\right) - 64\left(\frac{G^4}{r^6}\vec{S}_1\cdot\vec{n}\,\vec{S}_2\cdot\vec{n}\,m_1^3m_2^2\right), \tag{A.8}$$

$$\text{Fig. 2(b1.3)} = 5\left(\frac{G^4}{r^6}\vec{S}_1\cdot\vec{n}\,\vec{S}_2\cdot\vec{n}\,m_1^3m_2^2\right) - \left(\frac{G^4}{r^6}\vec{S}_1\cdot\vec{S}_2\,m_1^3m_2^2\right), \tag{A.9}$$

$$\text{Fig. 2(b1.4)} = -8\left(\frac{G^4}{r^6}\vec{S}_1\cdot\vec{n}\,\vec{S}_2\cdot\vec{n}\,m_1^3m_2^2\right), \tag{A.10}$$

$$\text{Fig. 2(b2.1)} = 8\left(\frac{G^4}{r^6}\vec{S}_1\cdot\vec{S}_2\,m_1^3m_2^2\right) - 16\left(\frac{G^4}{r^6}\vec{S}_1\cdot\vec{n}\,\vec{S}_2\cdot\vec{n}\,m_1^3m_2^2\right), \tag{A.11}$$

$$\text{Fig. 2(b2.2)} = -8\left(\frac{G^4}{r^6}\vec{S}_1\cdot\vec{n}\,\vec{S}_2\cdot\vec{n}\,m_1^3m_2^2\right), \tag{A.12}$$

$$\text{Fig. 2(b3.1)} = 8\left(\frac{G^4}{r^6}\vec{S}_1\cdot\vec{S}_2\,m_1^3m_2^2\right) - 16\left(\frac{G^4}{r^6}\vec{S}_1\cdot\vec{n}\,\vec{S}_2\cdot\vec{n}\,m_1^3m_2^2\right), \tag{A.13}$$

$$\text{Fig. 2(b3.2)} = 10\left(\frac{G^4}{r^6}\vec{S}_1\cdot\vec{n}\,\vec{S}_2\cdot\vec{n}\,m_1^3m_2^2\right) - 2\left(\frac{G^4}{r^6}\vec{S}_1\cdot\vec{S}_2\,m_1^3m_2^2\right), \tag{A.14}$$

$$\text{Fig. 2(b4.1)} = 8\left(\frac{G^4}{r^6}\vec{S}_1\cdot\vec{S}_2\,m_1^3m_2^2\right) - 16\left(\frac{G^4}{r^6}\vec{S}_1\cdot\vec{n}\,\vec{S}_2\cdot\vec{n}\,m_1^3m_2^2\right), \tag{A.15}$$

$$\text{Fig. 2(b4.2)} = 2\left(\frac{G^4}{r^6}\vec{S}_1\cdot\vec{S}_2\,m_1^3m_2^2\right) - 4\left(\frac{G^4}{r^6}\vec{S}_1\cdot\vec{n}\,\vec{S}_2\cdot\vec{n}\,m_1^3m_2^2\right), \tag{A.16}$$

$$\text{Fig. 2(b4.3)} = -32\left(\frac{G^4}{r^6}\vec{S}_1\cdot\vec{n}\,\vec{S}_2\cdot\vec{n}\,m_1^3m_2^2\right), \tag{A.17}$$

$$\text{Fig. 2(b5.1)} = 16\left(\frac{G^4}{r^6}\vec{S}_1\cdot\vec{S}_2\,m_1^4m_2\right) - 32\left(\frac{G^4}{r^6}\vec{S}_1\cdot\vec{n}\,\vec{S}_2\cdot\vec{n}\,m_1^4m_2\right), \tag{A.18}$$

$$\text{Fig. 2(b5.2)} = 10\left(\frac{G^4}{r^6}\vec{S}_1\cdot\vec{n}\,\vec{S}_2\cdot\vec{n}\,m_1^4m_2\right) - 2\left(\frac{G^4}{r^6}\vec{S}_1\cdot\vec{S}_2\,m_1^4m_2\right), \tag{A.19}$$

$$\text{Fig. 2(b6.1)} = \left(\frac{G^4}{r^6}\vec{S}_1\cdot\vec{S}_2\,m_1^3m_2^2\right) - 2\left(\frac{G^4}{r^6}\vec{S}_1\cdot\vec{n}\,\vec{S}_2\cdot\vec{n}\,m_1^3m_2^2\right), \tag{A.20}$$

$$\text{Fig. 2(b6.2)} = 16\left(\frac{G^4}{r^6}\vec{S}_1\cdot\vec{S}_2\, m_1^3 m_2^2\right) - 32\left(\frac{G^4}{r^6}\vec{S}_1\cdot\vec{n}\,\vec{S}_2\cdot\vec{n}\, m_1^3 m_2^2\right), \tag{A.21}$$

$$\text{Fig. 2(b6.3)} = -32\left(\frac{G^4}{r^6}\vec{S}_1\cdot\vec{n}\,\vec{S}_2\cdot\vec{n}\, m_1^3 m_2^2\right), \tag{A.22}$$

$$\text{Fig. 2(c1.1)} = 0, \tag{A.23}$$

$$\text{Fig. 2(c1.2)} = 0, \tag{A.24}$$

$$\text{Fig. 2(c2.1)} = \frac{96}{5}\left(\frac{G^4}{r^6}\vec{S}_1\cdot\vec{S}_2\, m_1^4 m_2\right) - 32\left(\frac{G^4}{r^6}\vec{S}_1\cdot\vec{n}\,\vec{S}_2\cdot\vec{n}\, m_1^4 m_2\right), \tag{A.25}$$

$$\text{Fig. 2(c3.1)} = \frac{96}{5}\left(\frac{G^4}{r^6}\vec{S}_1\cdot\vec{S}_2\, m_1^3 m_2^2\right) - 32\left(\frac{G^4}{r^6}\vec{S}_1\cdot\vec{n}\,\vec{S}_2\cdot\vec{n}\, m_1^3 m_2^2\right), \tag{A.26}$$

$$\text{Fig. 2(c3.2)} = \frac{48}{5}\left(\frac{G^4}{r^6}\vec{S}_1\cdot\vec{S}_2\, m_1^3 m_2^2\right) - 16\left(\frac{G^4}{r^6}\vec{S}_1\cdot\vec{n}\,\vec{S}_2\cdot\vec{n}\, m_1^3 m_2^2\right), \tag{A.27}$$

$$\text{Fig. 2(e1.1)} = 8\left(\frac{G^4}{r^6}\vec{S}_1\cdot\vec{n}\,\vec{S}_2\cdot\vec{n}\, m_1^3 m_2^2\right), \tag{A.28}$$

$$\text{Fig. 2(e1.2)} = \left(\frac{G^4}{r^6}\vec{S}_1\cdot\vec{S}_2\, m_1^3 m_2^2\right) - 3\left(\frac{G^4}{r^6}\vec{S}_1\cdot\vec{n}\,\vec{S}_2\cdot\vec{n}\, m_1^3 m_2^2\right), \tag{A.29}$$

$$\text{Fig. 2(e2.1)} = \left(\frac{G^4}{r^6}\vec{S}_1\cdot\vec{S}_2\, m_1^4 m_2\right) - 3\left(\frac{G^4}{r^6}\vec{S}_1\cdot\vec{n}\,\vec{S}_2\cdot\vec{n}\, m_1^4 m_2\right), \tag{A.30}$$

$$\text{Fig. 2(e3.1)} = 8\left(\frac{G^4}{r^6}\vec{S}_1\cdot\vec{n}\,\vec{S}_2\cdot\vec{n}\, m_1^3 m_2^2\right), \tag{A.31}$$

$$\text{Fig. 2(e4.1)} = 0, \tag{A.32}$$

$$\text{Fig. 2(e4.2)} = 0, \tag{A.33}$$

$$\text{Fig. 2(e4.3)} = 0, \tag{A.34}$$

$$\text{Fig. 2(e5.1)} = 48\left(\frac{G^4}{r^6}\vec{S}_1\cdot\vec{n}\,\vec{S}_2\cdot\vec{n}\, m_1^4 m_2\right) - \frac{144}{5}\left(\frac{G^4}{r^6}\vec{S}_1\cdot\vec{S}_2\, m_1^4 m_2\right), \tag{A.35}$$

$$\text{Fig. 2(e5.2)} = 4\left(\frac{G^4}{r^6}\vec{S}_1\cdot\vec{n}\,\vec{S}_2\cdot\vec{n}\, m_1^4 m_2\right) - \frac{4}{3}\left(\frac{G^4}{r^6}\vec{S}_1\cdot\vec{S}_2\, m_1^4 m_2\right), \tag{A.36}$$

$$\text{Fig. 2(e5.3)} = 4\left(\frac{G^4}{r^6}\vec{S}_1\cdot\vec{n}\,\vec{S}_2\cdot\vec{n}\, m_1^4 m_2\right) - \frac{12}{5}\left(\frac{G^4}{r^6}\vec{S}_1\cdot\vec{S}_2\, m_1^4 m_2\right), \tag{A.37}$$

$$\text{Fig. 2(e6.1)} = 12\left(\frac{G^4}{r^6}\vec{S}_1\cdot\vec{n}\,\vec{S}_2\cdot\vec{n}\, m_1^3 m_2^2\right) - \frac{36}{5}\left(\frac{G^4}{r^6}\vec{S}_1\cdot\vec{S}_2\, m_1^3 m_2^2\right), \tag{A.38}$$

$$\text{Fig. 2(e6.2)} = 4\left(\frac{G^4}{r^6}\vec{S}_1\cdot\vec{n}\,\vec{S}_2\cdot\vec{n}\, m_1^3 m_2^2\right) - \frac{4}{3}\left(\frac{G^4}{r^6}\vec{S}_1\cdot\vec{S}_2\, m_1^3 m_2^2\right), \tag{A.39}$$

$$\text{Fig. 2(e6.3)} = 4\left(\frac{G^4}{r^6}\vec{S}_1\cdot\vec{n}\,\vec{S}_2\cdot\vec{n}\, m_1^3 m_2^2\right) - \frac{12}{5}\left(\frac{G^4}{r^6}\vec{S}_1\cdot\vec{S}_2\, m_1^3 m_2^2\right), \tag{A.40}$$

$$\text{Fig. 2(e7.1)} = 48\left(\frac{G^4}{r^6}\vec{S}_1\cdot\vec{n}\,\vec{S}_2\cdot\vec{n}\, m_1^3 m_2^2\right) - \frac{144}{5}\left(\frac{G^4}{r^6}\vec{S}_1\cdot\vec{S}_2\, m_1^3 m_2^2\right), \tag{A.41}$$

$$\text{Fig. 2(e7.2)} = 12\left(\frac{G^4}{r^6}\vec{S}_1\cdot\vec{n}\,\vec{S}_2\cdot\vec{n}\, m_1^3 m_2^2\right) - \frac{36}{5}\left(\frac{G^4}{r^6}\vec{S}_1\cdot\vec{S}_2\, m_1^3 m_2^2\right), \tag{A.42}$$

$$\text{Fig. 2(e7.3)} = 8\left(\frac{G^4}{r^6}\vec{S}_1\cdot\vec{n}\,\vec{S}_2\cdot\vec{n}\, m_1^3 m_2^2\right) - \frac{8}{3}\left(\frac{G^4}{r^6}\vec{S}_1\cdot\vec{S}_2\, m_1^3 m_2^2\right), \tag{A.43}$$

$$\text{Fig. 2(e7.4)} = 2\left(\frac{G^4}{r^6}\vec{S}_1\cdot\vec{n}\,\vec{S}_2\cdot\vec{n}\,m_1^3m_2^2\right) - \frac{6}{5}\left(\frac{G^4}{r^6}\vec{S}_1\cdot\vec{S}_2\,m_1^3m_2^2\right), \tag{A.44}$$

$$\text{Fig. 2(e8.1)} = 48\left(\frac{G^4}{r^6}\vec{S}_1\cdot\vec{n}\,\vec{S}_2\cdot\vec{n}\,m_1^3m_2^2\right) - 16\left(\frac{G^4}{r^6}\vec{S}_1\cdot\vec{S}_2\,m_1^3m_2^2\right), \tag{A.45}$$

$$\text{Fig. 2(e8.2)} = 12\left(\frac{G^4}{r^6}\vec{S}_1\cdot\vec{n}\,\vec{S}_2\cdot\vec{n}\,m_1^3m_2^2\right) - 4\left(\frac{G^4}{r^6}\vec{S}_1\cdot\vec{S}_2\,m_1^3m_2^2\right), \tag{A.46}$$

$$\text{Fig. 2(e8.3)} = 48\left(\frac{G^4}{r^6}\vec{S}_1\cdot\vec{n}\,\vec{S}_2\cdot\vec{n}\,m_1^3m_2^2\right) - 16\left(\frac{G^4}{r^6}\vec{S}_1\cdot\vec{S}_2\,m_1^3m_2^2\right), \tag{A.47}$$

$$\text{Fig. 2(e8.4)} = 200\left(\frac{G^4}{r^6}\vec{S}_1\cdot\vec{n}\,\vec{S}_2\cdot\vec{n}\,m_1^3m_2^2\right) - 40\left(\frac{G^4}{r^6}\vec{S}_1\cdot\vec{S}_2\,m_1^3m_2^2\right), \tag{A.48}$$

$$\text{Fig. 2(e8.5)} = 50\left(\frac{G^4}{r^6}\vec{S}_1\cdot\vec{n}\,\vec{S}_2\cdot\vec{n}\,m_1^3m_2^2\right) - 10\left(\frac{G^4}{r^6}\vec{S}_1\cdot\vec{S}_2\,m_1^3m_2^2\right) \tag{A.49}$$

$$\begin{aligned}\text{Fig. 3(d1.1)} = {}& \frac{96}{5}\left(\frac{G^4}{r^6}\vec{S}_1\cdot\vec{n}\,\vec{S}_2\cdot\vec{n}\,m_1^3m_2^2\left(\frac{1}{d-3} - 4\ln\left(\frac{r}{R_0}\right)\right)\right) \\ &+ \frac{1392}{25}\left(\frac{G^4}{r^6}\vec{S}_1\cdot\vec{n}\,\vec{S}_2\cdot\vec{n}\,m_1^3m_2^2\right) + \frac{272}{15}\left(\frac{G^4}{r^6}\vec{S}_1\cdot\vec{S}_2\,m_1^3m_2^2\right),\end{aligned} \tag{A.50}$$

$$\text{Fig. 3(d2.1)} = \frac{64}{9}\left(\frac{G^4}{r^6}\vec{S}_1\cdot\vec{S}_2\,m_1^4m_2\right) - \frac{32}{3}\left(\frac{G^4}{r^6}\vec{S}_1\cdot\vec{n}\,\vec{S}_2\cdot\vec{n}\,m_1^4m_2\right), \tag{A.51}$$

$$\begin{aligned}\text{Fig. 3(f1.1)} = {}& \frac{16}{5}\left(\frac{G^4}{r^6}\vec{S}_1\cdot\vec{n}\,\vec{S}_2\cdot\vec{n}\,m_1^3m_2^2\left(\frac{1}{d-3} - 4\ln\left(\frac{r}{R_0}\right)\right)\right) \\ &+ \frac{2176}{75}\left(\frac{G^4}{r^6}\vec{S}_1\cdot\vec{n}\,\vec{S}_2\cdot\vec{n}\,m_1^3m_2^2\right) - \frac{176}{5}\left(\frac{G^4}{r^6}\vec{S}_1\cdot\vec{S}_2\,m_1^3m_2^2\right) \\ &- \frac{16}{3}\left(\frac{G^4}{r^6}\vec{S}_1\cdot\vec{S}_2\,m_1^3m_2^2\left(\frac{1}{d-3} - 4\ln\left(\frac{r}{R_0}\right)\right)\right),\end{aligned} \tag{A.52}$$

$$\begin{aligned}\text{Fig. 3(f1.2)} = {}& \frac{28}{5}\left(\frac{G^4}{r^6}\vec{S}_1\cdot\vec{n}\,\vec{S}_2\cdot\vec{n}\,m_1^3m_2^2\left(\frac{1}{d-3} - 4\ln\left(\frac{r}{R_0}\right)\right)\right) \\ &+ \frac{2548}{75}\left(\frac{G^4}{r^6}\vec{S}_1\cdot\vec{n}\,\vec{S}_2\cdot\vec{n}\,m_1^3m_2^2\right) - \frac{38}{5}\left(\frac{G^4}{r^6}\vec{S}_1\cdot\vec{S}_2\,m_1^3m_2^2\right) \\ &- \frac{4}{3}\left(\frac{G^4}{r^6}\vec{S}_1\cdot\vec{S}_2\,m_1^3m_2^2\left(\frac{1}{d-3} - 4\ln\left(\frac{r}{R_0}\right)\right)\right),\end{aligned} \tag{A.53}$$

$$\begin{aligned}\text{Fig. 3(f2.1)} = {}& \frac{32}{5}\left(\frac{G^4}{r^6}\vec{S}_1\cdot\vec{n}\,\vec{S}_2\cdot\vec{n}\,m_1^3m_2^2\left(\frac{1}{d-3} - 4\ln\left(\frac{r}{R_0}\right)\right)\right) \\ &+ \frac{2672}{75}\left(\frac{G^4}{r^6}\vec{S}_1\cdot\vec{n}\,\vec{S}_2\cdot\vec{n}\,m_1^3m_2^2\right) - \frac{1808}{75}\left(\frac{G^4}{r^6}\vec{S}_1\cdot\vec{S}_2\,m_1^3m_2^2\right) \\ &- \frac{64}{15}\left(\frac{G^4}{r^6}\vec{S}_1\cdot\vec{S}_2\,m_1^3m_2^2\left(\frac{1}{d-3} - 4\ln\left(\frac{r}{R_0}\right)\right)\right),\end{aligned} \tag{A.54}$$

$$\text{Fig. 3(f3.1)} = \frac{64}{3}\left(\frac{G^4}{r^6}\vec{S}_1\cdot\vec{n}\,\vec{S}_2\cdot\vec{n}\,m_1^4m_2\right) - \frac{128}{9}\left(\frac{G^4}{r^6}\vec{S}_1\cdot\vec{S}_2\,m_1^4m_2\right), \tag{A.55}$$

$$\text{Fig. 3(f3.2)} = \frac{8}{3}\left(\frac{G^4}{r^6}\vec{S}_1\cdot\vec{n}\,\vec{S}_2\cdot\vec{n}\,m_1^4m_2\right) - \frac{16}{9}\left(\frac{G^4}{r^6}\vec{S}_1\cdot\vec{S}_2\,m_1^4m_2\right), \tag{A.56}$$

$$\text{Fig. 3(f4.1)} = \frac{416}{15}\left(\frac{G^4}{r^6}\vec{S}_1\cdot\vec{n}\,\vec{S}_2\cdot\vec{n}\,m_1^4m_2\right) - \frac{832}{45}\left(\frac{G^4}{r^6}\vec{S}_1\cdot\vec{S}_2\,m_1^4m_2\right), \tag{A.57}$$

$$\begin{aligned}\text{Fig. 3(f5.1)} = &-\frac{208}{5}\left(\frac{G^4}{r^6}\vec{S}_1\cdot\vec{n}\,\vec{S}_2\cdot\vec{n}\,m_1^3m_2^2\left(\frac{1}{d-3}-4\ln\left(\frac{r}{R_0}\right)\right)\right)\\ &-\frac{9688}{75}\left(\frac{G^4}{r^6}\vec{S}_1\cdot\vec{n}\,\vec{S}_2\cdot\vec{n}\,m_1^3m_2^2\right)-\frac{8}{3}\left(\frac{G^4}{r^6}\vec{S}_1\cdot\vec{S}_2\,m_1^3m_2^2\right)\\ &+\frac{16}{3}\left(\frac{G^4}{r^6}\vec{S}_1\cdot\vec{S}_2\,m_1^3m_2^2\left(\frac{1}{d-3}-4\ln\left(\frac{r}{R_0}\right)\right)\right),\end{aligned} \tag{A.58}$$

$$\begin{aligned}\text{Fig. 3(f5.2)} = &-\frac{224}{5}\left(\frac{G^4}{r^6}\vec{S}_1\cdot\vec{n}\,\vec{S}_2\cdot\vec{n}\,m_1^3m_2^2\left(\frac{1}{d-3}-4\ln\left(\frac{r}{R_0}\right)\right)\right)\\ &-\frac{10184}{75}\left(\frac{G^4}{r^6}\vec{S}_1\cdot\vec{n}\,\vec{S}_2\cdot\vec{n}\,m_1^3m_2^2\right)-\frac{184}{25}\left(\frac{G^4}{r^6}\vec{S}_1\cdot\vec{S}_2\,m_1^3m_2^2\right)\\ &+\frac{64}{15}\left(\frac{G^4}{r^6}\vec{S}_1\cdot\vec{S}_2\,m_1^3m_2^2\left(\frac{1}{d-3}-4\ln\left(\frac{r}{R_0}\right)\right)\right),\end{aligned} \tag{A.59}$$

$$\begin{aligned}\text{Fig. 3(f5.3)} = &-38\left(\frac{G^4}{r^6}\vec{S}_1\cdot\vec{n}\,\vec{S}_2\cdot\vec{n}\,m_1^3m_2^2\left(\frac{1}{d-3}-4\ln\left(\frac{r}{R_0}\right)\right)\right)\\ &-\frac{502}{3}\left(\frac{G^4}{r^6}\vec{S}_1\cdot\vec{n}\,\vec{S}_2\cdot\vec{n}\,m_1^3m_2^2\right)+\frac{81\pi^2}{4}\left(\frac{G^4}{r^6}\vec{S}_1\cdot\vec{n}\,\vec{S}_2\cdot\vec{n}\,m_1^3m_2^2\right)\\ &+\frac{34}{3}\left(\frac{G^4}{r^6}\vec{S}_1\cdot\vec{S}_2\,m_1^3m_2^2\left(\frac{1}{d-3}-4\ln\left(\frac{r}{R_0}\right)\right)\right)\\ &+58\left(\frac{G^4}{r^6}\vec{S}_1\cdot\vec{S}_2\,m_1^3m_2^2\right)-\frac{27\pi^2}{4}\left(\frac{G^4}{r^6}\vec{S}_1\cdot\vec{S}_2\,m_1^3m_2^2\right),\end{aligned} \tag{A.60}$$

$$\begin{aligned}\text{Fig. 3(g1.1)} = &-\frac{4}{5}\left(\frac{G^4}{r^6}\vec{S}_1\cdot\vec{n}\,\vec{S}_2\cdot\vec{n}\,m_1^3m_2^2\left(\frac{1}{d-3}-4\ln\left(\frac{r}{R_0}\right)\right)\right)\\ &-\frac{544}{75}\left(\frac{G^4}{r^6}\vec{S}_1\cdot\vec{n}\,\vec{S}_2\cdot\vec{n}\,m_1^3m_2^2\right)+\frac{122}{25}\left(\frac{G^4}{r^6}\vec{S}_1\cdot\vec{S}_2\,m_1^3m_2^2\right)\\ &+\frac{8}{15}\left(\frac{G^4}{r^6}\vec{S}_1\cdot\vec{S}_2\,m_1^3m_2^2\left(\frac{1}{d-3}-4\ln\left(\frac{r}{R_0}\right)\right)\right),\end{aligned} \tag{A.61}$$

$$\begin{aligned}\text{Fig. 3(g1.2)} = &-\frac{48}{5}\left(\frac{G^4}{r^6}\vec{S}_1\cdot\vec{n}\,\vec{S}_2\cdot\vec{n}\,m_1^3m_2^2\left(\frac{1}{d-3}-4\ln\left(\frac{r}{R_0}\right)\right)\right)\\ &-\frac{1376}{25}\left(\frac{G^4}{r^6}\vec{S}_1\cdot\vec{n}\,\vec{S}_2\cdot\vec{n}\,m_1^3m_2^2\right)+\frac{2792}{75}\left(\frac{G^4}{r^6}\vec{S}_1\cdot\vec{S}_2\,m_1^3m_2^2\right)\\ &+\frac{32}{5}\left(\frac{G^4}{r^6}\vec{S}_1\cdot\vec{S}_2\,m_1^3m_2^2\left(\frac{1}{d-3}-4\ln\left(\frac{r}{R_0}\right)\right)\right),\end{aligned} \tag{A.62}$$

$$\text{Fig. 3(g2.1)} = \frac{4}{9}\left(\frac{G^4}{r^6}\vec{S}_1\cdot\vec{S}_2\,m_1^4m_2\right) - \frac{2}{3}\left(\frac{G^4}{r^6}\vec{S}_1\cdot\vec{n}\,\vec{S}_2\cdot\vec{n}\,m_1^4m_2\right), \tag{A.63}$$

$$\text{Fig. 3(g3.1)} = \frac{8}{9}\left(\frac{G^4}{r^6}\vec{S}_1\cdot\vec{S}_2\,m_1^4m_2\right) - \frac{4}{3}\left(\frac{G^4}{r^6}\vec{S}_1\cdot\vec{n}\,\vec{S}_2\cdot\vec{n}\,m_1^4m_2\right), \tag{A.64}$$

$$\text{Fig. 3(g3.2)} = \frac{104}{45}\left(\frac{G^4}{r^6}\vec{S}_1\cdot\vec{S}_2\,m_1^4m_2\right) - \frac{52}{15}\left(\frac{G^4}{r^6}\vec{S}_1\cdot\vec{n}\,\vec{S}_2\cdot\vec{n}\,m_1^4m_2\right), \tag{A.65}$$

$$\text{Fig. 3(g3.3)} = \frac{416}{15}\left(\frac{G^4}{r^6}\vec{S}_1\cdot\vec{S}_2\, m_1^4 m_2\right) - \frac{208}{5}\left(\frac{G^4}{r^6}\vec{S}_1\cdot\vec{n}\,\vec{S}_2\cdot\vec{n}\, m_1^4 m_2\right), \tag{A.66}$$

$$\begin{aligned}\text{Fig. 3(g4.1)} = {} & 14\left(\frac{G^4}{r^6}\vec{S}_1\cdot\vec{n}\,\vec{S}_2\cdot\vec{n}\, m_1^3 m_2^2\left(\frac{1}{d-3} - 4\ln\left(\frac{r}{R_0}\right)\right)\right) \\ & + \frac{214}{3}\left(\frac{G^4}{r^6}\vec{S}_1\cdot\vec{n}\,\vec{S}_2\cdot\vec{n}\, m_1^3 m_2^2\right) - \frac{27\pi^2}{4}\left(\frac{G^4}{r^6}\vec{S}_1\cdot\vec{n}\,\vec{S}_2\cdot\vec{n}\, m_1^3 m_2^2\right) \\ & - \frac{10}{3}\left(\frac{G^4}{r^6}\vec{S}_1\cdot\vec{S}_2\, m_1^3 m_2^2\left(\frac{1}{d-3} - 4\ln\left(\frac{r}{R_0}\right)\right)\right) \\ & - 18\left(\frac{G^4}{r^6}\vec{S}_1\cdot\vec{S}_2\, m_1^3 m_2^2\right) + \frac{9\pi^2}{4}\left(\frac{G^4}{r^6}\vec{S}_1\cdot\vec{S}_2\, m_1^3 m_2^2\right),\end{aligned} \tag{A.67}$$

$$\begin{aligned}\text{Fig. 3(g4.2)} = {} & \frac{24}{5}\left(\frac{G^4}{r^6}\vec{S}_1\cdot\vec{n}\,\vec{S}_2\cdot\vec{n}\, m_1^3 m_2^2\left(\frac{1}{d-3} - 4\ln\left(\frac{r}{R_0}\right)\right)\right) \\ & + \frac{288}{25}\left(\frac{G^4}{r^6}\vec{S}_1\cdot\vec{n}\,\vec{S}_2\cdot\vec{n}\, m_1^3 m_2^2\right) + \frac{968}{75}\left(\frac{G^4}{r^6}\vec{S}_1\cdot\vec{S}_2\, m_1^3 m_2^2\right) \\ & + \frac{8}{5}\left(\frac{G^4}{r^6}\vec{S}_1\cdot\vec{S}_2\, m_1^3 m_2^2\left(\frac{1}{d-3} - 4\ln\left(\frac{r}{R_0}\right)\right)\right),\end{aligned} \tag{A.68}$$

$$\begin{aligned}\text{Fig. 3(g4.3)} = {} & -\frac{22}{5}\left(\frac{G^4}{r^6}\vec{S}_1\cdot\vec{n}\,\vec{S}_2\cdot\vec{n}\, m_1^3 m_2^2\left(\frac{1}{d-3} - 4\ln\left(\frac{r}{R_0}\right)\right)\right) \\ & - \frac{1867}{75}\left(\frac{G^4}{r^6}\vec{S}_1\cdot\vec{n}\,\vec{S}_2\cdot\vec{n}\, m_1^3 m_2^2\right) + \frac{413}{75}\left(\frac{G^4}{r^6}\vec{S}_1\cdot\vec{S}_2\, m_1^3 m_2^2\right) \\ & + \frac{14}{15}\left(\frac{G^4}{r^6}\vec{S}_1\cdot\vec{S}_2\, m_1^3 m_2^2\left(\frac{1}{d-3} - 4\ln\left(\frac{r}{R_0}\right)\right)\right),\end{aligned} \tag{A.69}$$

$$\begin{aligned}\text{Fig. 3(g4.4)} = {} & -\frac{2}{5}\left(\frac{G^4}{r^6}\vec{S}_1\cdot\vec{n}\,\vec{S}_2\cdot\vec{n}\, m_1^3 m_2^2\left(\frac{1}{d-3} - 4\ln\left(\frac{r}{R_0}\right)\right)\right) \\ & - \frac{287}{75}\left(\frac{G^4}{r^6}\vec{S}_1\cdot\vec{n}\,\vec{S}_2\cdot\vec{n}\, m_1^3 m_2^2\right) - \frac{49}{75}\left(\frac{G^4}{r^6}\vec{S}_1\cdot\vec{S}_2\, m_1^3 m_2^2\right) \\ & - \frac{2}{15}\left(\frac{G^4}{r^6}\vec{S}_1\cdot\vec{S}_2\, m_1^3 m_2^2\left(\frac{1}{d-3} - 4\ln\left(\frac{r}{R_0}\right)\right)\right),\end{aligned} \tag{A.70}$$

$$\begin{aligned}\text{Fig. 3(g5.1)} = {} & \frac{8}{5}\left(\frac{G^4}{r^6}\vec{S}_1\cdot\vec{n}\,\vec{S}_2\cdot\vec{n}\, m_1^3 m_2^2\left(\frac{1}{d-3} - 4\ln\left(\frac{r}{R_0}\right)\right)\right) \\ & - \frac{292}{75}\left(\frac{G^4}{r^6}\vec{S}_1\cdot\vec{n}\,\vec{S}_2\cdot\vec{n}\, m_1^3 m_2^2\right) - \frac{9\pi^2}{4}\left(\frac{G^4}{r^6}\vec{S}_1\cdot\vec{n}\,\vec{S}_2\cdot\vec{n}\, m_1^3 m_2^2\right) \\ & - \frac{16}{15}\left(\frac{G^4}{r^6}\vec{S}_1\cdot\vec{S}_2\, m_1^3 m_2^2\left(\frac{1}{d-3} - 4\ln\left(\frac{r}{R_0}\right)\right)\right) \\ & + \frac{248}{75}\left(\frac{G^4}{r^6}\vec{S}_1\cdot\vec{S}_2\, m_1^3 m_2^2\right) + \frac{3\pi^2}{4}\left(\frac{G^4}{r^6}\vec{S}_1\cdot\vec{S}_2\, m_1^3 m_2^2\right),\end{aligned} \tag{A.71}$$

$$\begin{aligned}\text{Fig. 3(g5.2)} = {} & \frac{112}{5}\left(\frac{G^4}{r^6}\vec{S}_1\cdot\vec{n}\,\vec{S}_2\cdot\vec{n}\, m_1^3 m_2^2\left(\frac{1}{d-3} - 4\ln\left(\frac{r}{R_0}\right)\right)\right) \\ & + \frac{1342}{75}\left(\frac{G^4}{r^6}\vec{S}_1\cdot\vec{n}\,\vec{S}_2\cdot\vec{n}\, m_1^3 m_2^2\right) - \frac{45\pi^2}{4}\left(\frac{G^4}{r^6}\vec{S}_1\cdot\vec{n}\,\vec{S}_2\cdot\vec{n}\, m_1^3 m_2^2\right)\end{aligned} \tag{A.72}$$

$$-\frac{104}{15}\left(\frac{G^4}{r^6}\vec{S}_1\cdot\vec{S}_2\,m_1^3m_2^2\left(\frac{1}{d-3}-4\ln\left(\frac{r}{R_0}\right)\right)\right)$$
$$-\frac{366}{25}\left(\frac{G^4}{r^6}\vec{S}_1\cdot\vec{S}_2\,m_1^3m_2^2\right)+\frac{15\pi^2}{4}\left(\frac{G^4}{r^6}\vec{S}_1\cdot\vec{S}_2\,m_1^3m_2^2\right),$$

$$\text{Fig. 3(g5.3)}=\frac{312}{5}\left(\frac{G^4}{r^6}\vec{S}_1\cdot\vec{n}\,\vec{S}_2\cdot\vec{n}\,m_1^3m_2^2\left(\frac{1}{d-3}-4\ln\left(\frac{r}{R_0}\right)\right)\right) \tag{A.73}$$
$$+\frac{4504}{25}\left(\frac{G^4}{r^6}\vec{S}_1\cdot\vec{n}\,\vec{S}_2\cdot\vec{n}\,m_1^3m_2^2\right)+\frac{64}{15}\left(\frac{G^4}{r^6}\vec{S}_1\cdot\vec{S}_2\,m_1^3m_2^2\right)$$
$$-8\left(\frac{G^4}{r^6}\vec{S}_1\cdot\vec{S}_2\,m_1^3m_2^2\left(\frac{1}{d-3}-4\ln\left(\frac{r}{R_0}\right)\right)\right)$$

$$\text{Fig. 4(b1.1)}=8\left(\frac{G^4}{r^6}\left(\vec{S}_1\cdot\vec{n}\right)^2m_1^3m_2^2\right), \tag{A.74}$$

$$\text{Fig. 4(b2.1)}=16\left(\frac{G^4}{r^6}\left(\vec{S}_1\cdot\vec{n}\right)^2m_1^2m_2^3\right), \tag{A.75}$$

$$\text{Fig. 4(b3.1)}=\left(\frac{G^4}{r^6}\left(\vec{S}_1\cdot\vec{n}\right)^2m_1^3m_2^2\right), \tag{A.76}$$

$$\text{Fig. 4(b4.1)}=8\left(\frac{G^4}{r^6}\left(\vec{S}_1\cdot\vec{n}\right)^2m_1^3m_2^2\right), \tag{A.77}$$

$$\text{Fig. 4(b5.1)}=\frac{1}{2}\left(\frac{G^4}{r^6}\left(\vec{S}_1\cdot\vec{n}\right)^2m_1^4m_2\right), \tag{A.78}$$

$$\text{Fig. 4(b6.1)}=16\left(\frac{G^4}{r^6}\left(\vec{S}_1\cdot\vec{n}\right)^2m_1^2m_2^3\right), \tag{A.79}$$

$$\text{Fig. 4(c1.1)}=0, \tag{A.80}$$

$$\text{Fig. 4(c1.2)}=0, \tag{A.81}$$

$$\text{Fig. 4(c2.1)}=\frac{12}{7}\left(\frac{G^4}{r^6}\left(\vec{S}_1\cdot\vec{n}\right)^2m_1^4m_2\right)+\frac{8}{35}\left(\frac{G^4}{r^6}S_1^2\,m_1^4m_2\right), \tag{A.82}$$

$$\text{Fig. 4(c3.1)}=\frac{96}{7}\left(\frac{G^4}{r^6}\left(\vec{S}_1\cdot\vec{n}\right)^2m_1^3m_2^2\right)+\frac{64}{35}\left(\frac{G^4}{r^6}S_1^2\,m_1^3m_2^2\right), \tag{A.83}$$

$$\text{Fig. 4(c3.2)}=\frac{12}{7}\left(\frac{G^4}{r^6}\left(\vec{S}_1\cdot\vec{n}\right)^2m_1^3m_2^2\right)+\frac{8}{35}\left(\frac{G^4}{r^6}S_1^2\,m_1^3m_2^2\right), \tag{A.84}$$

$$\text{Fig. 4(e1.1)}=2\left(\frac{G^4}{r^6}\left(\vec{S}_1\cdot\vec{n}\right)^2m_1^2m_2^3\right), \tag{A.85}$$

$$\text{Fig. 4(e3.1)}=-8\left(\frac{G^4}{r^6}\left(\vec{S}_1\cdot\vec{n}\right)^2m_1^3m_2^2\right), \tag{A.86}$$

$$\text{Fig. 4(e4.1)}=0, \tag{A.87}$$

$$\text{Fig. 4(e4.2)}=0, \tag{A.88}$$

$$\text{Fig. 4(e5.1)}=-\frac{4}{7}\left(\frac{G^4}{r^6}\left(\vec{S}_1\cdot\vec{n}\right)^2m_1^4m_2\right)-\frac{12}{35}\left(\frac{G^4}{r^6}S_1^2\,m_1^4m_2\right), \tag{A.89}$$

$$\text{Fig. 4(e5.2)}=\frac{13}{70}\left(\frac{G^4}{r^6}S_1^2\,m_1^4m_2\right)-\frac{5}{14}\left(\frac{G^4}{r^6}\left(\vec{S}_1\cdot\vec{n}\right)^2m_1^4m_2\right), \tag{A.90}$$

$$\text{Fig. 4(e6.1)} = -\frac{16}{7}\left(\frac{G^4}{r^6}\left(\vec{S}_1\cdot\vec{n}\right)^2 m_1^3 m_2^2\right) - \frac{48}{35}\left(\frac{G^4}{r^6}S_1^2\, m_1^3 m_2^2\right), \tag{A.91}$$

$$\text{Fig. 4(e6.2)} = \frac{13}{70}\left(\frac{G^4}{r^6}S_1^2\, m_1^3 m_2^2\right) - \frac{5}{14}\left(\frac{G^4}{r^6}\left(\vec{S}_1\cdot\vec{n}\right)^2 m_1^3 m_2^2\right), \tag{A.92}$$

$$\text{Fig. 4(e7.1)} = -\frac{16}{7}\left(\frac{G^4}{r^6}\left(\vec{S}_1\cdot\vec{n}\right)^2 m_1^3 m_2^2\right) - \frac{48}{35}\left(\frac{G^4}{r^6}S_1^2\, m_1^3 m_2^2\right), \tag{A.93}$$

$$\text{Fig. 4(e7.2)} = -\frac{4}{7}\left(\frac{G^4}{r^6}\left(\vec{S}_1\cdot\vec{n}\right)^2 m_1^3 m_2^2\right) - \frac{12}{35}\left(\frac{G^4}{r^6}S_1^2\, m_1^3 m_2^2\right), \tag{A.94}$$

$$\text{Fig. 4(e7.3)} = \frac{52}{35}\left(\frac{G^4}{r^6}S_1^2\, m_1^3 m_2^2\right) - \frac{20}{7}\left(\frac{G^4}{r^6}\left(\vec{S}_1\cdot\vec{n}\right)^2 m_1^3 m_2^2\right), \tag{A.95}$$

$$\text{Fig. 4(e8.1)} = 0, \tag{A.96}$$

$$\text{Fig. 4(e8.2)} = 0 \tag{A.97}$$

$$\begin{aligned}\text{Fig. 5(d1.1)} = {} & 8\left(\frac{G^4}{r^6}\left(\vec{S}_1\cdot\vec{n}\right)^2 m_1^2 m_2^3\left(\frac{1}{d-3} - 4\ln\left(\frac{r}{R_0}\right)\right)\right) \\ & + \frac{76}{3}\left(\frac{G^4}{r^6}\left(\vec{S}_1\cdot\vec{n}\right)^2 m_1^2 m_2^3\right) + \frac{68}{3}\left(\frac{G^4}{r^6}S_1^2\, m_1^2 m_2^3\right) \\ & + \frac{8}{3}\left(\frac{G^4}{r^6}S_1^2\, m_1^2 m_2^3\left(\frac{1}{d-3} - 4\ln\left(\frac{r}{R_0}\right)\right)\right),\end{aligned} \tag{A.98}$$

$$\begin{aligned}\text{Fig. 5(d1.2)} = {} & \frac{192}{35}\left(\frac{G^4}{r^6}\left(\vec{S}_1\cdot\vec{n}\right)^2 m_1^3 m_2^2\left(\frac{1}{d-3} - 4\ln\left(\frac{r}{R_0}\right)\right)\right) \\ & + \frac{19968}{1225}\left(\frac{G^4}{r^6}\left(\vec{S}_1\cdot\vec{n}\right)^2 m_1^3 m_2^2\right) + \frac{45776}{3675}\left(\frac{G^4}{r^6}S_1^2\, m_1^3 m_2^2\right) \\ & + \frac{48}{35}\left(\frac{G^4}{r^6}S_1^2\, m_1^3 m_2^2\left(\frac{1}{d-3} - 4\ln\left(\frac{r}{R_0}\right)\right)\right),\end{aligned} \tag{A.99}$$

$$\text{Fig. 5(d2.1)} = 2\left(\frac{G^4}{r^6}\left(\vec{S}_1\cdot\vec{n}\right)^2 m_1^4 m_2\right) + \frac{2}{5}\left(\frac{G^4}{r^6}S_1^2\, m_1^4 m_2\right), \tag{A.100}$$

$$\begin{aligned}\text{Fig. 5(f1.1)} = {} & -\frac{64}{35}\left(\frac{G^4}{r^6}\left(\vec{S}_1\cdot\vec{n}\right)^2 m_1^3 m_2^2\left(\frac{1}{d-3} - 4\ln\left(\frac{r}{R_0}\right)\right)\right) \\ & - \frac{14368}{3675}\left(\frac{G^4}{r^6}\left(\vec{S}_1\cdot\vec{n}\right)^2 m_1^3 m_2^2\right) - \frac{8704}{735}\left(\frac{G^4}{r^6}S_1^2\, m_1^3 m_2^2\right) \\ & - \frac{32}{21}\left(\frac{G^4}{r^6}S_1^2\, m_1^3 m_2^2\left(\frac{1}{d-3} - 4\ln\left(\frac{r}{R_0}\right)\right)\right),\end{aligned} \tag{A.101}$$

$$\begin{aligned}\text{Fig. 5(f1.2)} = {} & \left(\frac{G^4}{r^6}\left(\vec{S}_1\cdot\vec{n}\right)^2 m_1^2 m_2^3\left(\frac{1}{d-3} - 4\ln\left(\frac{r}{R_0}\right)\right)\right) \\ & + \frac{8}{3}\left(\frac{G^4}{r^6}\left(\vec{S}_1\cdot\vec{n}\right)^2 m_1^2 m_2^3\right) + \frac{8}{3}\left(\frac{G^4}{r^6}S_1^2\, m_1^2 m_2^3\right) \\ & + \frac{1}{3}\left(\frac{G^4}{r^6}S_1^2\, m_1^2 m_2^3\left(\frac{1}{d-3} - 4\ln\left(\frac{r}{R_0}\right)\right)\right),\end{aligned} \tag{A.102}$$

$$\text{Fig. 5(f2.1)} = \frac{1}{7}\left(\frac{G^4}{r^6}\left(\vec{S}_1\cdot\vec{n}\right)^2 m_1^3 m_2^2\left(\frac{1}{d-3} - 4\ln\left(\frac{r}{R_0}\right)\right)\right) \tag{A.103}$$

$$+\frac{281}{1470}\left(\frac{G^4}{r^6}\left(\vec{S}_1\cdot\vec{n}\right)^2 m_1^3m_2^2\right)+\frac{179}{490}\left(\frac{G^4}{r^6}S_1^2\,m_1^3m_2^2\right)$$

$$+\frac{1}{21}\left(\frac{G^4}{r^6}S_1^2\,m_1^3m_2^2\left(\frac{1}{d-3}-4\ln\left(\frac{r}{R_0}\right)\right)\right),$$

$$\text{Fig. 5(f3.1)}=-\frac{4}{3}\left(\frac{G^4}{r^6}\left(\vec{S}_1\cdot\vec{n}\right)^2 m_1^4m_2\right)-\frac{44}{45}\left(\frac{G^4}{r^6}S_1^2\,m_1^4m_2\right), \tag{A.104}$$

$$\text{Fig. 5(f3.2)}=\frac{1}{3}\left(\frac{G^4}{r^6}\left(\vec{S}_1\cdot\vec{n}\right)^2 m_1^4m_2\right)-\frac{1}{45}\left(\frac{G^4}{r^6}S_1^2\,m_1^4m_2\right), \tag{A.105}$$

$$\text{Fig. 5(f4.1)}=-\frac{4}{15}\left(\frac{G^4}{r^6}\left(\vec{S}_1\cdot\vec{n}\right)^2 m_1^4m_2\right)-\frac{28}{45}\left(\frac{G^4}{r^6}S_1^2\,m_1^4m_2\right), \tag{A.106}$$

$$\text{Fig. 5(f4.2)}=\frac{12}{35}\left(\frac{G^4}{r^6}\left(\vec{S}_1\cdot\vec{n}\right)^2 m_1^4m_2\left(\frac{1}{d-3}-4\ln\left(\frac{r}{R_0}\right)\right)\right) \tag{A.107}$$

$$+\frac{10393}{7350}\left(\frac{G^4}{r^6}\left(\vec{S}_1\cdot\vec{n}\right)^2 m_1^4m_2\right)-\frac{7733}{22050}\left(\frac{G^4}{r^6}S_1^2\,m_1^4m_2\right)$$

$$-\frac{4}{35}\left(\frac{G^4}{r^6}S_1^2\,m_1^4m_2\left(\frac{1}{d-3}-4\ln\left(\frac{r}{R_0}\right)\right)\right),$$

$$\text{Fig. 5(f5.1)}=-32\left(\frac{G^4}{r^6}\left(\vec{S}_1\cdot\vec{n}\right)^2 m_1^2m_2^3\left(\frac{1}{d-3}-4\ln\left(\frac{r}{R_0}\right)\right)\right) \tag{A.108}$$

$$-\frac{256}{3}\left(\frac{G^4}{r^6}\left(\vec{S}_1\cdot\vec{n}\right)^2 m_1^2m_2^3\right)-\frac{256}{3}\left(\frac{G^4}{r^6}S_1^2\,m_1^2m_2^3\right) \tag{A.109}$$

$$-\frac{32}{3}\left(\frac{G^4}{r^6}S_1^2\,m_1^2m_2^3\left(\frac{1}{d-3}-4\ln\left(\frac{r}{R_0}\right)\right)\right),$$

$$\text{Fig. 5(f5.2)}=-\frac{704}{35}\left(\frac{G^4}{r^6}\left(\vec{S}_1\cdot\vec{n}\right)^2 m_1^3m_2^2\left(\frac{1}{d-3}-4\ln\left(\frac{r}{R_0}\right)\right)\right) \tag{A.110}$$

$$-\frac{179048}{3675}\left(\frac{G^4}{r^6}\left(\vec{S}_1\cdot\vec{n}\right)^2 m_1^3m_2^2\right)-\frac{45128}{1225}\left(\frac{G^4}{r^6}S_1^2\,m_1^3m_2^2\right)$$

$$-\frac{416}{105}\left(\frac{G^4}{r^6}S_1^2\,m_1^3m_2^2\left(\frac{1}{d-3}-4\ln\left(\frac{r}{R_0}\right)\right)\right),$$

$$\text{Fig. 5(f5.3)}=-\frac{62}{35}\left(\frac{G^4}{r^6}\left(\vec{S}_1\cdot\vec{n}\right)^2 m_1^3m_2^2\left(\frac{1}{d-3}-4\ln\left(\frac{r}{R_0}\right)\right)\right) \tag{A.111}$$

$$-\frac{44684}{3675}\left(\frac{G^4}{r^6}\left(\vec{S}_1\cdot\vec{n}\right)^2 m_1^3m_2^2\right)+\frac{21652}{3675}\left(\frac{G^4}{r^6}S_1^2\,m_1^3m_2^2\right)$$

$$+\frac{118}{105}\left(\frac{G^4}{r^6}S_1^2\,m_1^3m_2^2\left(\frac{1}{d-3}-4\ln\left(\frac{r}{R_0}\right)\right)\right),$$

$$\text{Fig. 5(g1.1)}=\left(\frac{G^4}{r^6}\left(\vec{S}_1\cdot\vec{n}\right)^2 m_1^2m_2^3\left(\frac{1}{d-3}-4\ln\left(\frac{r}{R_0}\right)\right)\right) \tag{A.112}$$

$$+\frac{17}{3}\left(\frac{G^4}{r^6}\left(\vec{S}_1\cdot\vec{n}\right)^2 m_1^2m_2^3\right)+\frac{11}{3}\left(\frac{G^4}{r^6}S_1^2\,m_1^2m_2^3\right)$$

$$+\frac{1}{3}\left(\frac{G^4}{r^6}S_1^2\,m_1^2m_2^3\left(\frac{1}{d-3}-4\ln\left(\frac{r}{R_0}\right)\right)\right),$$

$$\text{Fig. 5(g1.2)} = -\frac{2}{35}\left(\frac{G^4}{r^6}\left(\vec{S}_1\cdot\vec{n}\right)^2 m_1^3 m_2^2\left(\frac{1}{d-3}-4\ln\left(\frac{r}{R_0}\right)\right)\right) - \frac{169}{3675}\left(\frac{G^4}{r^6}\left(\vec{S}_1\cdot\vec{n}\right)^2 m_1^3 m_2^2\right) - \frac{4427}{11025}\left(\frac{G^4}{r^6}S_1^2\, m_1^3 m_2^2\right) - \frac{2}{35}\left(\frac{G^4}{r^6}S_1^2\, m_1^3 m_2^2\left(\frac{1}{d-3}-4\ln\left(\frac{r}{R_0}\right)\right)\right), \tag{A.113}$$

$$\text{Fig. 5(g1.3)} = -\frac{3}{35}\left(\frac{G^4}{r^6}\left(\vec{S}_1\cdot\vec{n}\right)^2 m_1^3 m_2^2\left(\frac{1}{d-3}-4\ln\left(\frac{r}{R_0}\right)\right)\right) - \frac{2537}{7350}\left(\frac{G^4}{r^6}\left(\vec{S}_1\cdot\vec{n}\right)^2 m_1^3 m_2^2\right) - \frac{671}{22050}\left(\frac{G^4}{r^6}S_1^2\, m_1^3 m_2^2\right) + \frac{1}{105}\left(\frac{G^4}{r^6}S_1^2\, m_1^3 m_2^2\left(\frac{1}{d-3}-4\ln\left(\frac{r}{R_0}\right)\right)\right), \tag{A.114}$$

$$\text{Fig. 5(g2.1)} = \frac{5}{6}\left(\frac{G^4}{r^6}\left(\vec{S}_1\cdot\vec{n}\right)^2 m_1^4 m_2\right) - \frac{1}{18}\left(\frac{G^4}{r^6}S_1^2\, m_1^4 m_2\right), \tag{A.115}$$

$$\text{Fig. 5(g2.2)} = \frac{4}{15}\left(\frac{G^4}{r^6}S_1^2\, m_1^4 m_2\right), \tag{A.116}$$

$$\text{Fig. 5(g3.1)} = \frac{1}{30}\left(\frac{G^4}{r^6}\left(\vec{S}_1\cdot\vec{n}\right)^2 m_1^4 m_2\right) + \frac{7}{90}\left(\frac{G^4}{r^6}S_1^2\, m_1^4 m_2\right), \tag{A.117}$$

$$\text{Fig. 5(g3.2)} = \frac{2}{5}\left(\frac{G^4}{r^6}\left(\vec{S}_1\cdot\vec{n}\right)^2 m_1^4 m_2\right) + \frac{14}{15}\left(\frac{G^4}{r^6}S_1^2\, m_1^4 m_2\right), \tag{A.118}$$

$$\text{Fig. 5(g3.3)} = -\frac{8}{35}\left(\frac{G^4}{r^6}\left(\vec{S}_1\cdot\vec{n}\right)^2 m_1^4 m_2\left(\frac{1}{d-3}-4\ln\left(\frac{r}{R_0}\right)\right)\right) - \frac{3791}{3675}\left(\frac{G^4}{r^6}\left(\vec{S}_1\cdot\vec{n}\right)^2 m_1^4 m_2\right) + \frac{3371}{11025}\left(\frac{G^4}{r^6}S_1^2\, m_1^4 m_2\right) + \frac{8}{105}\left(\frac{G^4}{r^6}S_1^2\, m_1^4 m_2\left(\frac{1}{d-3}-4\ln\left(\frac{r}{R_0}\right)\right)\right), \tag{A.119}$$

$$\text{Fig. 5(g3.4)} = -\frac{4}{35}\left(\frac{G^4}{r^6}\left(\vec{S}_1\cdot\vec{n}\right)^2 m_1^4 m_2\left(\frac{1}{d-3}-4\ln\left(\frac{r}{R_0}\right)\right)\right) - \frac{937}{2450}\left(\frac{G^4}{r^6}\left(\vec{S}_1\cdot\vec{n}\right)^2 m_1^4 m_2\right) + \frac{991}{22050}\left(\frac{G^4}{r^6}S_1^2\, m_1^4 m_2\right) + \frac{4}{105}\left(\frac{G^4}{r^6}S_1^2\, m_1^4 m_2\left(\frac{1}{d-3}-4\ln\left(\frac{r}{R_0}\right)\right)\right), \tag{A.120}$$

$$\text{Fig. 5(g4.1)} = -2\left(\frac{G^4}{r^6}\left(\vec{S}_1\cdot\vec{n}\right)^2 m_1^2 m_2^3\left(\frac{1}{d-3}-4\ln\left(\frac{r}{R_0}\right)\right)\right) - \frac{22}{3}\left(\frac{G^4}{r^6}\left(\vec{S}_1\cdot\vec{n}\right)^2 m_1^2 m_2^3\right) - 6\left(\frac{G^4}{r^6}S_1^2\, m_1^2 m_2^3\right) - \frac{2}{3}\left(\frac{G^4}{r^6}S_1^2\, m_1^2 m_2^3\left(\frac{1}{d-3}-4\ln\left(\frac{r}{R_0}\right)\right)\right), \tag{A.121}$$

$$\text{Fig. 5(g4.2)} = -4\left(\frac{G^4}{r^6}\left(\vec{S}_1\cdot\vec{n}\right)^2 m_1^3 m_2^2\left(\frac{1}{d-3}-4\ln\left(\frac{r}{R_0}\right)\right)\right) \tag{A.122}$$

$$- \frac{196}{15}\left(\frac{G^4}{r^6}\left(\vec{S}_1\cdot\vec{n}\right)^2 m_1^3 m_2^2\right) + \frac{9\pi^2}{8}\left(\frac{G^4}{r^6}\left(\vec{S}_1\cdot\vec{n}\right)^2 m_1^3 m_2^2\right)$$

$$+ \frac{8}{3}\left(\frac{G^4}{r^6} S_1^2\, m_1^3 m_2^2\left(\frac{1}{d-3} - 4\ln\left(\frac{r}{R_0}\right)\right)\right)$$

$$+ \frac{172}{15}\left(\frac{G^4}{r^6} S_1^2\, m_1^3 m_2^2\right) - \frac{3\pi^2}{8}\left(\frac{G^4}{r^6} S_1^2\, m_1^3 m_2^2\right),$$

$$\text{Fig. 5(g4.3)} = \frac{96}{35}\left(\frac{G^4}{r^6}\left(\vec{S}_1\cdot\vec{n}\right)^2 m_1^3 m_2^2\left(\frac{1}{d-3} - 4\ln\left(\frac{r}{R_0}\right)\right)\right) + \frac{4664}{1225}\left(\frac{G^4}{r^6}\left(\vec{S}_1\cdot\vec{n}\right)^2 m_1^3 m_2^2\right) + \frac{11992}{735}\left(\frac{G^4}{r^6} S_1^2\, m_1^3 m_2^2\right) + \frac{16}{7}\left(\frac{G^4}{r^6} S_1^2\, m_1^3 m_2^2\left(\frac{1}{d-3} - 4\ln\left(\frac{r}{R_0}\right)\right)\right), \tag{A.123}$$

$$\text{Fig. 5(g5.1)} = \frac{202}{35}\left(\frac{G^4}{r^6}\left(\vec{S}_1\cdot\vec{n}\right)^2 m_1^3 m_2^2\left(\frac{1}{d-3} - 4\ln\left(\frac{r}{R_0}\right)\right)\right) + \frac{168514}{3675}\left(\frac{G^4}{r^6}\left(\vec{S}_1\cdot\vec{n}\right)^2 m_1^3 m_2^2\right) - \frac{9\pi^2}{8}\left(\frac{G^4}{r^6}\left(\vec{S}_1\cdot\vec{n}\right)^2 m_1^3 m_2^2\right) - \frac{398}{105}\left(\frac{G^4}{r^6} S_1^2\, m_1^3 m_2^2\left(\frac{1}{d-3} - 4\ln\left(\frac{r}{R_0}\right)\right)\right) - \frac{71422}{3675}\left(\frac{G^4}{r^6} S_1^2\, m_1^3 m_2^2\right) + \frac{3\pi^2}{8}\left(\frac{G^4}{r^6} S_1^2\, m_1^3 m_2^2\right), \tag{A.124}$$

$$\text{Fig. 5(g5.2)} = \frac{96}{7}\left(\frac{G^4}{r^6}\left(\vec{S}_1\cdot\vec{n}\right)^2 m_1^3 m_2^2\left(\frac{1}{d-3} - 4\ln\left(\frac{r}{R_0}\right)\right)\right) + \frac{9004}{245}\left(\frac{G^4}{r^6}\left(\vec{S}_1\cdot\vec{n}\right)^2 m_1^3 m_2^2\right) + \frac{74848}{3675}\left(\frac{G^4}{r^6} S_1^2\, m_1^3 m_2^2\right) + \frac{64}{35}\left(\frac{G^4}{r^6} S_1^2\, m_1^3 m_2^2\left(\frac{1}{d-3} - 4\ln\left(\frac{r}{R_0}\right)\right)\right), \tag{A.125}$$

$$\text{Fig. 5(g5.3)} = 24\left(\frac{G^4}{r^6}\left(\vec{S}_1\cdot\vec{n}\right)^2 m_1^2 m_2^3\left(\frac{1}{d-3} - 4\ln\left(\frac{r}{R_0}\right)\right)\right) + 56\left(\frac{G^4}{r^6}\left(\vec{S}_1\cdot\vec{n}\right)^2 m_1^2 m_2^3\right) + \frac{184}{3}\left(\frac{G^4}{r^6} S_1^2\, m_1^2 m_2^3\right) + 8\left(\frac{G^4}{r^6} S_1^2\, m_1^2 m_2^3\left(\frac{1}{d-3} - 4\ln\left(\frac{r}{R_0}\right)\right)\right) \tag{A.126}$$

$$\text{Fig. 6(a1.1)} = 12\left(C_{1ES^2}\frac{G^4}{r^6}\left(\vec{S}_1\cdot\vec{n}\right)^2 m_1^2 m_2^3\right) - 4\left(C_{1ES^2}\frac{G^4}{r^6} S_1^2\, m_1^2 m_2^3\right), \tag{A.127}$$

$$\text{Fig. 6(a1.2)} = \frac{3}{2}\left(C_{1ES^2}\frac{G^4}{r^6}\left(\vec{S}_1\cdot\vec{n}\right)^2 m_1^3 m_2^2\right) - \frac{1}{2}\left(C_{1ES^2}\frac{G^4}{r^6} S_1^2\, m_1^3 m_2^2\right), \tag{A.128}$$

$$\text{Fig. 6(a1.3)} = 6\left(C_{1ES^2}\frac{G^4}{r^6}\left(\vec{S}_1\cdot\vec{n}\right)^2 m_1^3 m_2^2\right) - 2\left(C_{1ES^2}\frac{G^4}{r^6} S_1^2\, m_1^3 m_2^2\right), \tag{A.129}$$

$$\text{Fig. 6(a2.1)} = \frac{135}{4}\left(C_{1ES^2}\frac{G^4}{r^6}\left(\vec{S}_1\cdot\vec{n}\right)^2 m_1^2 m_2^3\right) - \frac{45}{4}\left(C_{1ES^2}\frac{G^4}{r^6} S_1^2\, m_1^2 m_2^3\right), \tag{A.130}$$

$$\text{Fig. 6(a2.2)} = \frac{3}{4}\left(C_{1ES^2}\frac{G^4}{r^6}\left(\vec{S}_1\cdot\vec{n}\right)^2 m_1^2 m_2^3\right) - \frac{1}{4}\left(C_{1ES^2}\frac{G^4}{r^6}S_1^2\, m_1^2 m_2^3\right), \tag{A.131}$$

$$\text{Fig. 6(a2.3)} = \frac{3}{2}\left(C_{1ES^2}\frac{G^4}{r^6}\left(\vec{S}_1\cdot\vec{n}\right)^2 m_1^3 m_2^2\right) - \frac{1}{2}\left(C_{1ES^2}\frac{G^4}{r^6}S_1^2\, m_1^3 m_2^2\right), \tag{A.132}$$

$$\text{Fig. 6(a2.4)} = 6\left(C_{1ES^2}\frac{G^4}{r^6}\left(\vec{S}_1\cdot\vec{n}\right)^2 m_1^3 m_2^2\right) - 2\left(C_{1ES^2}\frac{G^4}{r^6}S_1^2\, m_1^3 m_2^2\right), \tag{A.133}$$

$$\text{Fig. 6(a3.1)} = \frac{27}{2}\left(C_{1ES^2}\frac{G^4}{r^6}\left(\vec{S}_1\cdot\vec{n}\right)^2 m_1 m_2^4\right) - \frac{9}{2}\left(C_{1ES^2}\frac{G^4}{r^6}S_1^2\, m_1 m_2^4\right), \tag{A.134}$$

$$\text{Fig. 6(a3.2)} = \frac{1}{4}\left(C_{1ES^2}\frac{G^4}{r^6}\left(\vec{S}_1\cdot\vec{n}\right)^2 m_1^4 m_2\right) - \frac{1}{12}\left(C_{1ES^2}\frac{G^4}{r^6}S_1^2\, m_1^4 m_2\right), \tag{A.135}$$

$$\text{Fig. 6(b1.1)} = \left(C_{1ES^2}\frac{G^4}{r^6}\left(\vec{S}_1\cdot\vec{n}\right)^2 m_1^2 m_2^3\right) + \left(C_{1ES^2}\frac{G^4}{r^6}S_1^2\, m_1^2 m_2^3\right), \tag{A.136}$$

$$\text{Fig. 6(b1.2)} = 3\left(C_{1ES^2}\frac{G^4}{r^6}\left(\vec{S}_1\cdot\vec{n}\right)^2 m_1^3 m_2^2\right) - 5\left(C_{1ES^2}\frac{G^4}{r^6}S_1^2\, m_1^3 m_2^2\right), \tag{A.137}$$

$$\text{Fig. 6(b2.1)} = 3\left(C_{1ES^2}\frac{G^4}{r^6}\left(\vec{S}_1\cdot\vec{n}\right)^2 m_1^2 m_2^3\right) - 5\left(C_{1ES^2}\frac{G^4}{r^6}S_1^2\, m_1^2 m_2^3\right), \tag{A.138}$$

$$\text{Fig. 6(b3.1)} = \frac{1}{2}\left(C_{1ES^2}\frac{G^4}{r^6}\left(\vec{S}_1\cdot\vec{n}\right)^2 m_1^2 m_2^3\right) + \frac{1}{2}\left(C_{1ES^2}\frac{G^4}{r^6}S_1^2\, m_1^2 m_2^3\right), \tag{A.139}$$

$$\text{Fig. 6(b4.1)} = 3\left(C_{1ES^2}\frac{G^4}{r^6}\left(\vec{S}_1\cdot\vec{n}\right)^2 m_1^3 m_2^2\right) - 5\left(C_{1ES^2}\frac{G^4}{r^6}S_1^2\, m_1^3 m_2^2\right), \tag{A.140}$$

$$\text{Fig. 6(b5.1)} = \frac{3}{2}\left(C_{1ES^2}\frac{G^4}{r^6}\left(\vec{S}_1\cdot\vec{n}\right)^2 m_1 m_2^4\right) + \frac{3}{2}\left(C_{1ES^2}\frac{G^4}{r^6}S_1^2\, m_1 m_2^4\right), \tag{A.141}$$

$$\text{Fig. 6(b6.1)} = 15\left(C_{1ES^2}\frac{G^4}{r^6}\left(\vec{S}_1\cdot\vec{n}\right)^2 m_1^2 m_2^3\right) - 17\left(C_{1ES^2}\frac{G^4}{r^6}S_1^2\, m_1^2 m_2^3\right), \tag{A.142}$$

$$\text{Fig. 6(e4.1)} = 0, \tag{A.143}$$

$$\text{Fig. 6(e4.2)} = 0, \tag{A.144}$$

$$\text{Fig. 6(e4.3)} = 0, \tag{A.145}$$

$$\text{Fig. 6(e4.4)} = 0, \tag{A.146}$$

$$\text{Fig. 6(e5.1)} = 12\left(C_{1ES^2}\frac{G^4}{r^6}\left(\vec{S}_1\cdot\vec{n}\right)^2 m_1 m_2^4\right) - 6\left(C_{1ES^2}\frac{G^4}{r^6}S_1^2\, m_1 m_2^4\right), \tag{A.147}$$

$$\text{Fig. 6(e5.2)} = \frac{1}{2}\left(C_{1ES^2}\frac{G^4}{r^6}\left(\vec{S}_1\cdot\vec{n}\right)^2 m_1^4 m_2\right) - \frac{1}{6}\left(C_{1ES^2}\frac{G^4}{r^6}S_1^2\, m_1^4 m_2\right), \tag{A.148}$$

$$\text{Fig. 6(e5.3)} = \frac{9}{7}\left(C_{1ES^2}\frac{G^4}{r^6}\left(\vec{S}_1\cdot\vec{n}\right)^2 m_1^4 m_2\right) - \frac{3}{7}\left(C_{1ES^2}\frac{G^4}{r^6}S_1^2\, m_1^4 m_2\right), \tag{A.149}$$

$$\text{Fig. 6(e5.4)} = \frac{3}{7}\left(C_{1ES^2}\frac{G^4}{r^6}\left(\vec{S}_1\cdot\vec{n}\right)^2 m_1^4 m_2\right) - \frac{1}{7}\left(C_{1ES^2}\frac{G^4}{r^6}S_1^2\, m_1^4 m_2\right), \tag{A.150}$$

$$\text{Fig. 6(e6.1)} = \frac{1}{2}\left(C_{1ES^2}\frac{G^4}{r^6}\left(\vec{S}_1\cdot\vec{n}\right)^2 m_1^2 m_2^3\right) - \frac{1}{6}\left(C_{1ES^2}\frac{G^4}{r^6}S_1^2\, m_1^2 m_2^3\right), \tag{A.151}$$

$$\text{Fig. 6(e6.2)} = \frac{5}{2}\left(C_{1ES^2}\frac{G^4}{r^6}\left(\vec{S}_1\cdot\vec{n}\right)^2 m_1^2 m_2^3\right) - \frac{3}{2}\left(C_{1ES^2}\frac{G^4}{r^6}S_1^2\, m_1^2 m_2^3\right), \tag{A.152}$$

$$\text{Fig. 6(e6.3)} = \frac{501}{70}\left(C_{1ES^2}\frac{G^4}{r^6}\left(\vec{S}_1\cdot\vec{n}\right)^2 m_1^3 m_2^2\right) - \frac{167}{70}\left(C_{1ES^2}\frac{G^4}{r^6}S_1^2\, m_1^3 m_2^2\right), \tag{A.153}$$

$$\text{Fig. 6(e6.4)} = \frac{3}{7}\left(C_{1ES^2}\frac{G^4}{r^6}\left(\vec{S}_1\cdot\vec{n}\right)^2 m_1^3 m_2^2\right) - \frac{1}{7}\left(C_{1ES^2}\frac{G^4}{r^6}S_1^2\, m_1^3 m_2^2\right), \tag{A.154}$$

$$\text{Fig. 6(e7.1)} = 5\left(C_{1ES^2}\frac{G^4}{r^6}\left(\vec{S}_1\cdot\vec{n}\right)^2 m_1^2 m_2^3\right) - 3\left(C_{1ES^2}\frac{G^4}{r^6}S_1^2\, m_1^2 m_2^3\right), \tag{A.155}$$

$$\text{Fig. 6(e7.2)} = \left(C_{1ES^2}\frac{G^4}{r^6}\left(\vec{S}_1\cdot\vec{n}\right)^2 m_1^2 m_2^3\right) - \frac{1}{3}\left(C_{1ES^2}\frac{G^4}{r^6}S_1^2\, m_1^2 m_2^3\right), \tag{A.156}$$

$$\text{Fig. 6(e7.3)} = \frac{18}{7}\left(C_{1ES^2}\frac{G^4}{r^6}\left(\vec{S}_1\cdot\vec{n}\right)^2 m_1^3 m_2^2\right) - \frac{6}{7}\left(C_{1ES^2}\frac{G^4}{r^6}S_1^2\, m_1^3 m_2^2\right), \tag{A.157}$$

$$\text{Fig. 6(e7.4)} = \frac{3}{7}\left(C_{1ES^2}\frac{G^4}{r^6}\left(\vec{S}_1\cdot\vec{n}\right)^2 m_1^3 m_2^2\right) - \frac{1}{7}\left(C_{1ES^2}\frac{G^4}{r^6}S_1^2\, m_1^3 m_2^2\right), \tag{A.158}$$

$$\text{Fig. 6(e7.5)} = \frac{192}{35}\left(C_{1ES^2}\frac{G^4}{r^6}\left(\vec{S}_1\cdot\vec{n}\right)^2 m_1^3 m_2^2\right) - \frac{64}{35}\left(C_{1ES^2}\frac{G^4}{r^6}S_1^2\, m_1^3 m_2^2\right), \tag{A.159}$$

$$\text{Fig. 6(e8.1)} = 81\left(C_{1ES^2}\frac{G^4}{r^6}\left(\vec{S}_1\cdot\vec{n}\right)^2 m_1^2 m_2^3\right) - 15\left(C_{1ES^2}\frac{G^4}{r^6}S_1^2\, m_1^2 m_2^3\right), \tag{A.160}$$

$$\text{Fig. 6(e8.2)} = 15\left(C_{1ES^2}\frac{G^4}{r^6}\left(\vec{S}_1\cdot\vec{n}\right)^2 m_1^2 m_2^3\right) - \left(C_{1ES^2}\frac{G^4}{r^6}S_1^2\, m_1^2 m_2^3\right), \tag{A.161}$$

$$\text{Fig. 6(e8.3)} = 6\left(C_{1ES^2}\frac{G^4}{r^6}\left(\vec{S}_1\cdot\vec{n}\right)^2 m_1^3 m_2^2\right) - 2\left(C_{1ES^2}\frac{G^4}{r^6}S_1^2\, m_1^3 m_2^2\right), \tag{A.162}$$

$$\text{Fig. 6(e8.4)} = 15\left(C_{1ES^2}\frac{G^4}{r^6}\left(\vec{S}_1\cdot\vec{n}\right)^2 m_1^3 m_2^2\right) - \left(C_{1ES^2}\frac{G^4}{r^6}S_1^2\, m_1^3 m_2^2\right), \tag{A.163}$$

$$\text{Fig. 6(e8.5)} = 15\left(C_{1ES^2}\frac{G^4}{r^6}\left(\vec{S}_1\cdot\vec{n}\right)^2 m_1^3 m_2^2\right) - \left(C_{1ES^2}\frac{G^4}{r^6}S_1^2\, m_1^3 m_2^2\right). \tag{A.164}$$
